# Supplementary material for: Incompressible Even Denominator Fractional Quantum Hall States in the Zeroth Landau Level of Monolayer Graphene
Source: arXiv:1809.07349 ancillary file (2018-09-25)
Supplement: Supplementary file 1 [file Supplement_arxiv.pdf]

# Supplementary material for "Incompressible Even Denominator Fractional Quantum Hall States in the Zeroth Landau Level of Monolayer Graphene"

Sujit Narayanan,[1] Bitan Roy,[2] and Malcolm P. Kennett[1]

[1]*Department of Physics, Simon Fraser University, 8888 University Drive, Burnaby, British Columbia, V5A 1S6, Canada.*

[2]*Max-Planck-Institut für Physik komplexer Systeme, Nöthnitzer Stra. 38, 01187 Dresden, Germany*

In these "Supplementary Materials", we present additional details, mainly pertaining to the equations that need to be solved to find the filling fraction and the corresponding order parameters for different choices of flux attachment.

## I. EQUATIONS RELATING ORDER PARAMETERS AND FILLING FRACTIONS

When we assume the $K$ matrix satisfies $k_1 = k_2$, $k_3 = k_4$, $n_1 = n_2 = n_3 = n_4$, then the equations we obtain by combining Eqs. (2) and (3) from the main text take the form

$$\begin{aligned}
\frac{4\nu_*}{\nu} &= 4 + [(2k_1 + m_1 + 2n)(\nu_1 + \nu_2) + (\nu_3 + \nu_4)(2k_3 + 2n + m_2)] \\
&+ C[(\nu_1 + \nu_2)(2k_1 + m_1 - 2n) - (\nu_3 + \nu_4)(2k_3 + m_2 - 2n)] \\
&+ F[(\nu_1 - \nu_2)(2k_1 - m_1) - (\nu_3 - \nu_4)(2k_3 - m_2)] + N[(\nu_1 - \nu_2)(2k_1 - m_1) - (\nu_3 - \nu_4)(2k_3 - m_2)], \quad (1) \\
\frac{4\nu_C}{\nu} &= 4C + [(2k_1 + m_1 + 2n)(\nu_1 + \nu_2) - (\nu_3 + \nu_4)(2k_3 + 2n + m_2)] \\
&+ C[(\nu_1 + \nu_2)(2k_1 + m_1 - 2n) + (\nu_3 + \nu_4)(2k_3 + m_2 - 2n)] \\
&+ F[(\nu_1 - \nu_2)(2k_1 - m_1) - (\nu_3 - \nu_4)(2k_3 - m_2)] + N[(\nu_1 - \nu_2)(2k_1 - m_1) + (\nu_3 - \nu_4)(2k_3 - m_2)], \quad (2) \\
\frac{4\nu_F}{\nu} &= 4F + [(2k_1 + m_1 + 2n)(\nu_1 - \nu_2) + (\nu_3 - \nu_4)(2k_3 + 2n + m_2)] \\
&+ C[(\nu_1 - \nu_2)(2k_1 + m_1 - 2n) - (\nu_3 - \nu_4)(2k_3 + m_2 - 2n)] \\
&+ F[(\nu_1 + \nu_2)(2k_1 - m_1) + (\nu_3 + \nu_4)(2k_3 - m_2)] + N[(\nu_1 + \nu_2)(2k_1 - m_1) - (\nu_3 + \nu_4)(2k_3 - m_2)], \quad (3) \\
\frac{4\nu_N}{\nu} &= 4N + [(2k_1 + m_1 + 2n)(\nu_1 - \nu_2) - (\nu_3 - \nu_4)(2k_3 + 2n + m_2)] \\
&+ C[(\nu_1 - \nu_2)(2k_1 + m_1 - 2n) + (\nu_3 - \nu_4)(2k_3 + m_2 - 2n)] \\
&+ F[(\nu_1 + \nu_2)(2k_1 - m_1) - (\nu_3 + \nu_4)(2k_3 - m_2)] + N[(\nu_1 + \nu_2)(2k_1 - m_1) + (\nu_3 + \nu_4)(2k_3 - m_2)], \quad (4)
\end{aligned}$$

which can be put in the form of Eq. (5) of the main text. The matrix $M$ can be read off from Eqs. (1)-(4). Assuming that $M$ is non-singular we can take the inverse to obtain

$$\begin{pmatrix} 1 \\ C \\ F \\ N \end{pmatrix} = \frac{1}{\nu} M^{-1} \begin{pmatrix} \nu_* \\ \nu_C \\ \nu_F \\ \nu_N \end{pmatrix},$$

with

$$M^{-1} = \frac{1}{\det(M)} \begin{pmatrix} b_{11} & b_{21} & b_{31} & b_{41} \\ b_{12} & b_{22} & b_{32} & b_{42} \\ b_{13} & b_{23} & b_{33} & b_{43} \\ b_{14} & b_{24} & b_{34} & b_{44} \end{pmatrix},$$

where $b_{ij}$ is the cofactor of $M_{ij}$.

Using the above relation we have

$$\begin{aligned}
\nu &= \frac{b_{11}\nu_* + b_{21}\nu_C + b_{31}\nu_F + b_{41}\nu_N}{\det(\mathrm{M})}, \quad C = \frac{1}{\nu}\frac{b_{12}\nu_* + b_{22}\nu_C + b_{32}\nu_F + b_{42}\nu_N}{\det(\mathrm{M})}, \\
F &= \frac{1}{\nu}\frac{b_{13}\nu_* + b_{23}\nu_C + b_{33}\nu_F + b_{43}\nu_N}{\det(\mathrm{M})}, \quad N = \frac{1}{\nu}\frac{b_{14}\nu_* + b_{24}\nu_C + b_{34}\nu_F + b_{44}\nu_N}{\det(\mathrm{M})}. \quad (5)
\end{aligned}$$

Solutions can always be obtained in this way but are not always amenable to a compact analytic expression.

### A. $(k, 2k, n)$ states

For the states with flux attachment $(k, 2k, n)$ we have $k = k_1 = k_3$, $m = 2k$ and $n \neq 2k$ and Eqs. (1)-(4) take the simpler form

$$\begin{pmatrix} 1+q_0\nu_* & q_1\nu_C & 0 & 0 \\ q_0\nu_C & 1+\nu_* q_1 & 0 & 0 \\ q_0\nu_F & q_1\nu_N & 1 & 0 \\ q_0\nu_N & q_1\nu_F & 0 & 1 \end{pmatrix} \begin{pmatrix} 1 \\ C \\ F \\ N \end{pmatrix} = \frac{1}{\nu} \begin{pmatrix} \nu_* \\ \nu_C \\ \nu_F \\ \nu_N \end{pmatrix},$$

with

$$q_0 = k + \frac{n}{2}, \qquad q_1 = k - \frac{n}{2}. \tag{6}$$

These equations can be solved using Eq. (5). Note that $\nu$ is expressed in Eq. (7) of the main text and the order parameters are given by

$$C = \frac{\nu_C}{\nu_* + \left(k - \frac{n}{2}\right)\left({\nu_*}^2 - \nu_C^2\right)}, \quad F = \frac{\nu_F + \left(k - \frac{n}{2}\right)\left(\nu_*\nu_F - \nu_N\nu_C\right)}{\nu_* + \left(k - \frac{n}{2}\right)\left({\nu_*}^2 - \nu_C^2\right)}, \quad N = \frac{\nu_N + \left(k - \frac{n}{2}\right)\left(\nu_*\nu_N - \nu_F\nu_C\right)}{\nu_* + \left(k - \frac{n}{2}\right)\left({\nu_*}^2 - \nu_C^2\right)}. \tag{7}$$

We use slightly different notation, but these expressions are equivalent to Eq. (12) in Ref. [1].

### B. $(k, m, 2k)$ states

The states with flux attachment $(k, m, 2k)$ are those for which $2k = 2k_1 = 2k_3$, $n = 2k$ and $m \neq 2k$. In this case we can write:

$$\begin{aligned} \frac{\nu_*}{\nu} &= (1+q_0\nu_*) + Cq_1\nu_C + Fq_2\nu_F + Nq_2\nu_N, \quad & \frac{\nu_C}{\nu} &= q_0\nu_C + (1+q_1\nu_*)C + Fq_2\nu_N + Nq_2\nu_F, \\ \frac{\nu_F}{\nu} &= q_0\nu_F + q_1\nu_N C + F(1+q_2\nu_*) + Nq_2\nu_C, \quad & \frac{\nu_N}{\nu} &= q_0\nu_N + q_1\nu_F C + Fq_2\nu_C + N(1+q_2\nu_*), \end{aligned} \tag{8}$$

with

$$q_0 = \frac{3k}{2} + \frac{m}{4}, \quad q_1 = \frac{m}{4} - \frac{k}{2} = -q_2.$$

We can use the general solutions listed above, with the determinant of $M$ and co-factors listed below to determine the allowed fractions and order parameters. The cofactors are as follows

$$\begin{aligned}
b_{11} &= (1+q_1\nu_*)(1-q_1\nu_*)^2 + 2q_1^3\nu_N\nu_C\nu_F + q_1^2(\nu_F^2+\nu_N^2)(1-q_1\nu_*) - q_1^2\nu_C^2(1+q_1\nu_*), \\
b_{12} &= -q_1\nu_C(1-q_1\nu_*)^2 - 2q_1^2\nu_F\nu_F(1-q_1\nu_*) + q_1^3\nu_C(\nu_C^2 - \nu_F^2\nu_N^2), \\
b_{13} &= 2q_1^3\nu_*\nu_C\nu_N + q_1\nu_F(1+q_1\nu_*)(1-q_1\nu_*) - q_1^3\nu_F(\nu_C^2 - \nu_F^2\nu_N^2), \\
b_{14} &= q_1\nu_N(1+q_1\nu_*)(1-q_1\nu_*) - q_1^3\nu_N(\nu_C^2+\nu_F^2-\nu_N^2) + 2q_1^3\nu_*\nu_F\nu_C, \\
b_{21} &= -q_0\nu_C(1-q_1\nu_*)^2 - 2q_0q_1\nu_F\nu_N(1-q_1\nu_*) + q_0q_1^2\nu_C(\nu_C^2-\nu_F^2-\nu_N^2), \\
b_{22} &= (1+q_0\nu_*)(1-q_1\nu_*)^2 + q_0q_1^2\nu_F\nu_C\nu_N + q_0q_1(\nu_F^2+\nu_N^2)(1-q_1\nu_*) - q_1^2\nu_C^2(1+q_0\nu_*), \\
b_{23} &= q_1\nu_N(1+q_0\nu_*)(1-q_1\nu_*) - q_0q_1^2\nu_N(\nu_C^2+\nu_F^2-\nu_N^2) - q_0q_1\nu_F\nu_C(1-q_1\nu_*) + q_1^2\nu_C\nu_F(1+q_0\nu_*), \\
b_{24} &= q_1^2\nu_C\nu_N(1+q_0\nu_*) - q_0q_1\nu_C\nu_N(1-q_1\nu_*) - q_0q_1^2\nu_F(\nu_C^2-\nu_F^2+\nu_N^2) + q_1\nu_F(1+q_0\nu_*)(1-q_1\nu_*), \\
b_{31} &= -2q_0q_1^2\nu_*\nu_C\nu_N + q_0q_1^2\nu_F(\nu_C^2-\nu_F^2+\nu_N^2) - q_0\nu_F(1+q_1\nu_*)(1-q_1\nu_*), \\
b_{32} &= -q_1\nu_N(1+q_0\nu_*)(1-q_1\nu_*) + q_0q_1^2\nu_N(\nu_C^2+\nu_F^2-\nu_n^2) + q_0q_1\nu_C\nu_F(1-q_1\nu_*) - q_1^2\nu_C\nu_F(1+q_0\nu_*), \\
b_{33} &= (1+q_0\nu_*)(1+q_1\nu_*)(1-q_1\nu_*) - 2q_0q_1^2\nu_C\nu_F\nu_N + q_0q_1\nu_N^2(1+q_1\nu_*) - q_0q_1\nu_C^2(1-q_1\nu_*) + q_1^2\nu_F^2(1+q_0\nu_*), \\
b_{34} &= q_1\nu_C(1+q_0\nu_*)(1+q_1\nu_*) - q_0q_1\nu_F\nu_N(1+q_1\nu_*) - q_0q_1^2\nu_C(\nu_c^2-\nu_F^2-\nu_N^2) - q_1^2\nu_F\nu_N(1+q_0\nu_*), \\
b_{41} &= q_0q_1^2\nu_N(\nu_C^2+\nu_F^2-\nu_N^2) - q_0\nu_N(1+q_1\nu_*)(1-q_1\nu_*) - 2q_0q_1^2\nu_*\nu_C\nu_F(1+q_1\nu_*), \\
b_{42} &= -q_1^2\nu_C\nu_N(1+q_0\nu_*) + q_0q_1\nu_C\nu_N(1-q_1\nu_*) + q_0q_1^2\nu_F(\nu_C^2-\nu_F^2+\nu_N^2) - q_1\nu_F(1+q_0\nu_*)(1-q_1\nu*), \\
b_{43} &= q_1\nu_C(1+q_0\nu_*)(1+q_1\nu_*) - q_0q_1\nu_F\nu_N(1+q_1\nu_*) - q_0q_1^2\nu_C(\nu_C^2-\nu_F^2-\nu_N^2) - q_1^2\nu_F\nu_N(1+q_0\nu_*), \\
b_{44} &= (1+q_0\nu_*)(1+q_1\nu_*)(1-q_1\nu_*) - 2q_0q_1^2\nu_C\nu_N\nu_F + q_0q_1\nu_F^2(1+q_1\nu_*) - q_0q_1\nu_C^2(1-q_1\nu_*) + q_1^2\nu_N^2(1+q_0\nu_*),
\end{aligned}$$

and the determinant is given by

$$\begin{aligned}\det(M) \;=\; & (1+q_0\nu_*)(1+q_1\nu_*)(1-q_1\nu_*)^2 + q_1^3\nu_C\nu_F(\nu_F+\nu_N)(1+q_0\nu_*) + q_1^2(\nu_F^2+\nu_N^2)(1+q_0\nu_*)(1-q_1\nu_*) \\ & -q_1^2\nu_C^2(1+q_0\nu_*)(1+q_1\nu_*) - q_0q_1\nu_C^2(1-q_1\nu_*)^2 - 4q_0q_1^2\nu_C\nu_F\nu_N(1-q_1\nu_*) + q_0q_1^3(\nu_C^4+\nu_F^4+\nu_N^4) \\ & -2q_0q_1^3\nu_F^2\nu_N^2 + q_0q_1(\nu_F^2-\nu_F\nu_N+\nu_N^2)(1+q_1\nu_*)(1-q_1\nu_*) - 2q_0q_1^3\nu_C^2(\nu_F^2+\nu_N^2) + q_0q_1^2\nu_C\nu_F\nu_N(1+q_1\nu_*).\end{aligned} \quad (9)$$

## C. $(k,m,n)$ states

For general states with flux attachment $(k,m,n)$ we have three parameters, $k$, $m \neq 2k$ and $n \neq 2k$. In this case we can write

$$\begin{aligned}\frac{\nu_*}{\nu} &= (1+q_0)\nu_* + Cq_1\nu_C + Fq_2\nu_F + Nq_2\nu_N, & \frac{\nu_C}{\nu} &= q_0\nu_C + (1+q_1\nu_*)C + Fq_2\nu_N + Nq_2\nu_F, \\ \frac{\nu_F}{\nu} &= q_0\nu_F + q_1\nu_N C + F(1+q_2\nu_*) + Nq_2\nu_C, & \frac{\nu_N}{\nu} &= q_0\nu_N + q_1\nu_F C + Fq_2\nu_C + N(1+q_2\nu_*),\end{aligned} \quad (10)$$

where

$$q_0 = \frac{k}{2} + \frac{m}{4} + \frac{n}{2}, \quad q_1 = \frac{k}{2} + \frac{m}{4} - \frac{n}{2}, \quad q_2 = \frac{k}{2} - \frac{m}{4}.$$

We do not write out the solutions to these equations explicitly.

## D. $\nu = \frac{1}{4}$

As mentioned in the main text, we found that there are states with flux attachment $(k, 2k, n)$ and $(k, m, 2k)$ that allow for an even denominator fractional quantum Hall (EDFQH) state at $\nu = \frac{1}{4}$. We write out the fillings $(\nu_1, \nu_2, \nu_3, \nu_4)$ and order parameters associated with these states in Table I.

| $(k,m,n)$ | $(\nu_1,\nu_2,\nu_3,\nu_4)$ | $(C,F,N)$ | Other fractions |
|---|---|---|---|
| (2,4,3) | (1, 0, 1, 0) | (0, 1, 0) | $\mathbf{\frac{1}{5}, \frac{2}{9}, \frac{3}{13}}$ |
| | (1, 0, 0, 1) | (0, 0, 1) | |
| | (0, 1, 1, 0) | (0, 0, -1) | |
| | (0, 1, 0, 1) | (0, -1, 0) | |
| (2,3,4) | (1, 1, 0, 0) | (1, 0, 0) | $\mathbf{\frac{1}{5}, \frac{2}{9}, \frac{3}{13}, \frac{3}{11}}$ |
| | (0, 0, 1, 1) | (-1, 0, 0) | |
| | (1, 1, 1, 0) | (1, 0, 0) | |
| | (1, 1, 0, 1) | (1, 0, 0) | |
| | (1, 0, 1, 1) | (-1, 0, 0) | |
| | (0, 1, 1, 1) | (-1, 0, 0) | |
| (3,6,1) | (1, 0, 1, 0) | (0, 1, 0) | $\frac{1}{7}, \frac{2}{13}$ |
| | (1, 0, 0, 1) | (0, 0, 1) | |
| | (0, 1, 1, 0) | (0, 0, -1) | |
| | (0, 1, 0, 1) | (0, -1, 0) | |

Table I: Parameters for possible $(k, 2k, n)$ and $(k, m, 2k)$ $\nu = \frac{1}{4}$ states. Fractions observed in Ref. [2] are indicated in **bold**.

[1] S. Modak, S. S. Mandal, and K. Sengupta, Phys. Rev. B **84**, 165118 (2011).
[2] A. A. Zibrov, E. M. Spanton, H. Zhou, C. Kometter, T. Taniguchi, K. Watanabe, and A. F. Young, Nature Phys. **14**, 930 (2018).
